# Supplementary material for: Smooth Mathematical Function from Compact Neural Networks
Source: arXiv:2301.00181 source file (2022-12-31)
Supplement: Supplementary file 1 [file APPENDIX.pdf]

# A Appendix

The following dataset was created from the formula in the physics book of graduate school. The situation in the original problem and the answer to it are as follows.

"A spring is connected to a support at one end and has a mass $m$ attached at the other, where the spring constant is $k$ and the rest length is $L$. Neglecting the mass of the spring, what is the angular position $\theta$ of mass $m$ under the gravitational field as a function of time $t$?"

=> **answer** : $\theta = B\cos(\sqrt{\frac{kg}{kL+km}}t + \phi)$, where $B, \phi$ are constants of integration.

The formula $\theta = B\cos(\sqrt{\frac{kg}{kL+km}}t + \phi)$ was slightly modified and the following dataset is generated.

$$\mathcal{D} = \{(B_i, k_i, m_i, L_i, t_i, \phi_i, \theta_i) | \theta_i = \sqrt{B_i}\cos(\sqrt{\frac{k_i g + (B_i - 0.3)^2}{k_i L_i + k_i m_i}} t_i + \phi_i), B_i \in [0.5, 1.5], \\ k_i \in [2, 5], g = 9.8, m_i \in [0.5, 2.5], L_i \in [1, 4], t_i \in [0.1, 2], \phi_i \in [0, 0.78]\} \\ \sim \{(B_i, k_i, m_i, \mathcal{D}_{B_i, k_i, m_i})\}$$

When it was trained, all the input variables $B, k, m, L, t, \phi$ were normalized.

For each of $B$, $k$, and $m$, 10 points were uniformly selected to make 1000 meta parameter sets $\{(B_i, k_i, m_i)\}$ and, for each meta parameter point, task datasets $\mathcal{D}_{B_i, k_i, m_i} = \{(L_i, t_i, \phi_i, \theta_i)\}$ which has 35301 points are created by selecting uniform 21 points of $L$, uniform 41 points of $t$ and uniform 41 points of $\phi$. Among them, 100 random meta parameters were selected, and 640 points were selected for each task to be used as meta train dataset. The selected points are shown in Figure 3.

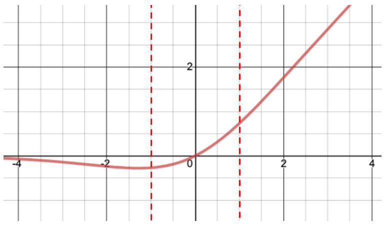

Figure 1: Swish.

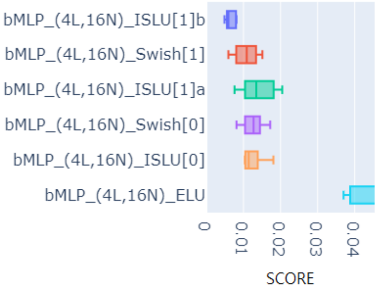


Figure 2: Points in train dataset.

# B Appendix

Swish also showed similar or sometimes slightly better performance than ISLU in the given experimental data. This is because Swish is good for generalization, and our data falls within the smoothed range of Swish activation in the range -1 to 1.

If the output data is in a range greater than -1 to 1, Swish may have to be used in a range that includes two bends, which may result in a slightly worse performance. In actual experiments, using Swish showed worse performance than ISLU if the output of the experimental data is greater than -1 to 1. Figure 7 shows the result of experiment with data obtained by increasing the function value by 20 times from the data in Appendix A, where bMLP means fMLP [1] with the new data .

# C Appendix

Even when comparing ISLU[0] and SoftPlus, there is a difference in performance. This is because the parameters try to follow a specific distribution when the natural network is trained.

[1]in **??**

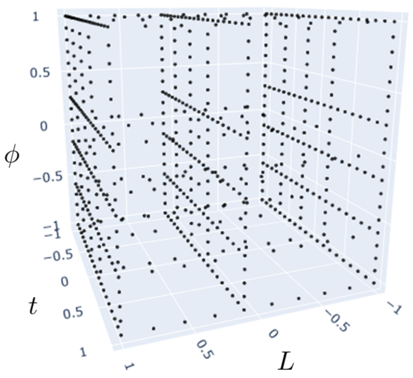


Figure 3: Points in train dataset.

In more detail, for two activation functions $AF$ and $AF' = AF + b$, when the parameter $w$ is multiplied, there is a difference in parallel movement by only $w * b$, since $w * AF'(x) = w * (AF(x) + b) = w * AF(x) + w * b$. It may be thought that the bias parameter will be adjusted to produce the same performance, but there is a difference in performance because the parameters of neural networks prefers a certain distribution. Furthermore, in the case of ISLU($x$,$\beta$) = SoftPlus($x$,$\beta$) + $b$($\beta$), the difference becomes larger because $\beta$ is entangled with translation part.

# D Appendix

Table 1: Table for Figure **??**

| Model | Score |
|---|---|
| MLP_(4L,64N)_ISLU[1]b | 0.0479 |
| MLP_(4L,64N)_ISLU[0] | 0.0650 |
| MLP_(4L,64N)_ELU | 0.0949 |
| MLP_(4L,64N)_ISLU[1]a | 0.1086 |
| MLP_(4L,16N)_ELU | 0.2673 |
| MLP_(4L,16N)_ISLU[0] | 0.3721 |
| MLP_(4L,16N)_ISLU[1]a | 0.3852 |
| MLP_(4L,16N)_SoftPlus[0] | 0.6512 |
| MLP_(4L,16N)_SoftPlus[1] | 1.5230 |
| MLP_(4L,16N)_ISLU[1]b | 14799.9303 |
| MLP_(4L,64N)_SoftPlus[0] | 314.3878 |
| MLP_(4L,64N)_SoftPlus[1] | 329.3783 |

Table 2: Table for Figure **??**

| Model | Score |
|---|---|
| fMLP_(4L,64N)_ISLU[0] | 0.0055 |
| fMLP_(4L,64N)_ISLU[1]a | 0.0062 |
| fMLP_(4L,16N)_ISLU[1]b | 0.0103 |
| fMLP_(4L,15N)_ISLU[1]b | 0.0112 |
| fMLP_(4L,16N)_ISLU[1]a | 0.0181 |
| fMLP_(4L,15N)_ISLU[1]a | 0.0191 |
| fMLP_(4L,16N)_ISLU[0] | 0.0247 |
| fMLP_(4L,64N)_SoftPlus[0] | 0.0418 |
| fMLP_(4L,64N)_SoftPlus[1] | 0.0438 |
| fMLP_(4L,64N)_ELU | 0.0691 |
| fMLP_(4L,16N)_ELU | 0.0793 |
| fMLP_(4L,16N)_SoftPlus[1] | 0.1306 |
| fMLP_(4L,16N)_SoftPlus[0] | 230.7397 |

Table 3: Table for Figure **??**

| Model | Score |
|---|---|
| WGN_(4L,64N)_ISLU[1]b_MB | 0.0023 |
| WGN_(4L,64N)_ISLU[0]_MB | 0.0024 |
| WGN_(4L,64N)_ISLU[1]a_MB | 0.0042 |
| WGN_(4L,16N)_ISLU[1]b_MB | 0.0057 |
| WGN_(4L,15N)_ISLU[1]b_MB | 0.0073 |
| WGN_(4L,16N)_ISLU[0]_MB | 0.0073 |
| WGN_(4L,15N)_ISLU[1]a_MB | 0.0077 |
| WGN_(4L,16N)_ISLU[1]a_MB | 0.0137 |
| WGN_(4L,64N)_ELU_MB | 0.0248 |
| WGN_(4L,16N)_ELU_MB | 0.0472 |

Table 4: Table for Figure **??**

| Model | Score |
|---|---|
| fMLP_(4L,64N)_ISLU[0] | 0.0055 |
| fMLP_(4L,16N)_ISLU[1]b | 0.0103 |
| fMLP_(4L,15N)_ISLU[1]b | 0.0112 |
| fMLP_(4L,16N)_ISLU[0] | 0.0247 |
| MLP_(4L,64N)_ISLU[1]b | 0.0479 |
| MLP_(4L,64N)_ISLU[0] | 0.0650 |
| fMLP_(4L,64N)_ELU | 0.0691 |
| fMLP_(4L,16N)_ELU | 0.0793 |
| MLP_(4L,64N)_ELU | 0.0949 |
| MLP_(4L,16N)_ELU | 0.2673 |
| MLP_(4L,16N)_ISLU[0] | 0.3721 |
| MLP_(4L,16N)_ISLU[1]b | 14799.9303 |

Table 5: Table for Figure **??**

| Model | Score |
|---|---|
| WGN_(4L,64N)_ISLU[1]b_MB | 0.0023 |
| WGN_(4L,16N)_ISLU[1]b_MB | 0.0057 |
| WGN_(4L,15N)_ISLU[1]b_MB | 0.0073 |
| WGN_(4L,64N)_ELU_MB | 0.0248 |
| WGN_(4L,64N)_ISLU[1]b_ST | 0.0330 |
| WGN_(4L,16N)_ELU_MB | 0.0472 |
| WGN_(4L,64N)_ELU_ST | 0.0487 |
| WGN_(4L,16N)_ISLU[1]b_ST | 0.2064 |
| WGN_(4L,16N)_ELU_ST | 0.3642 |

Table 6: Table for Figure **??**

| Model | Score |
|---|---|
| WGN_(4L,16N)_ISLU[1]b_MB | 0.0057 |
| WGN_(4L,16N)_ISLU[0]_MB | 0.0073 |
| WGN_(4L,16N)_ISLU[1]a_MB | 0.0137 |
| sWGN_(4L,16N)_ISLU[1]b_MB | 0.0161 |
| WGN_(4L,16N)_ELU_MB | 0.0472 |
| sWGN_(4L,16N)_ELU_MB | 0.0656 |
| mMLP_(4L,16N)_ISLU[1]b | 0.22439 |
| MLP_(4L,16N)_ELU | 0.26736 |
| MLP_(4L,16N)_ISLU[0] | 0.37218 |
| mMLP_(4L,16N)_ISLU[0] | 0.37807 |
| MLP_(4L,16N)_ISLU[1]a | 0.38529 |
| mMLP_(4L,16N)_ISLU[1]a | 0.58129 |
| mMLP_(4L,16N)_ELU | 0.86163 |
| MLP_(4L,16N)_ISLU[1]b | 14799.9303 |
